# Supplementary material for: Scale-invariant biomarker discovery in urine and plasma metabolite fingerprints
Source: arXiv:1703.07724 source file (2017-03-22)
Supplement: Supplementary file 1 [file supplement.pdf]

# Supplementary Material to Scale-invariant biomarker discovery in urine and plasma metabolite fingerprints

Helena U. Zacharias[1a,*], Thorsten Rehberg[b,*], Sebastian Mehrl[b], Daniel Richtmann[c], Tilo Wettig[c], Peter J. Oefner[a], Rainer Spang[b], Wolfram Gronwald[2a] and Michael Altenbuchinger[3b]

[a] *Institute of Functional Genomics, University of Regensburg, Regensburg, Germany*
[b] *Statistical Bioinformatics, Institute of Functional Genomics, University of Regensburg, Regensburg, Germany*
[c] *Department of Physics, University of Regensburg, Regensburg, Germany*

[*] The authors wish it to be known that, in their opinion, the first two authors should be regarded as Joint First Authors.

[1] helena.zacharias@ukr.de
[2] wolfram.gronwald@ukr.de
[3] michael.altenbuchinger@ukr.de

Table 1: Spectral positions and $p$-values of the ten most significant NMR buckets for the urinary AKI data set after (a) scaling to total spectral area, (b) scaling to creatinine, and (c) Probabilistic Quotient Normalization (PQN). The FDR was adjusted according to the method of Benjamini and Hochberg (B/H). In case more than one compound contributed to one significant bin, all possibly corresponding molecules are annotated.

**(a) scaling to total spectral area**

| **Spec. pos. [ppm]** | $\log_2$ **FC** | ***t*-value** | **raw *p*-value** | **B/H adj. *p*-value** | **Metabolite** |
|---|---|---|---|---|---|
| 2.465 | -1.02 | -6.59 | 1.53e-09 | 7.50e-07 | Carnitine/2-Oxoglutaric acid/Glutamine |
| 2.475 | -0.98 | -6.53 | 2.14e-09 | 7.50e-07 | Carnitine/Glutamine |
| 2.605 | -0.84 | -6.31 | 5.96e-09 | 1.39e-06 | Unknown |
| 2.385 | -0.87 | -6.22 | 9.16e-09 | 1.49e-06 | L-pyroglutamic acid/Unknown |
| 2.485 | -0.99 | -6.19 | 1.06e-08 | 1.49e-06 | Carnitine/Glutamine/Acetyl-L-carnitine |
| 2.245 | -1.01 | -6.12 | 1.46e-08 | 1.49e-06 | Unknown/Acetone |
| 2.365 | -0.87 | -6.12 | 1.49e-08 | 1.49e-06 | 3-Hydroxyisovaleric acid |
| 2.495 | -0.98 | -5.86 | 4.91e-08 | 4.29e-06 | Acetyl-L-carnitine/Glutamine/Unknown |
| 2.625 | -0.86 | -5.72 | 9.24e-08 | 7.18e-06 | Acetyl-L-carnitine |
| 3.235 | -1.13 | -5.68 | 1.13e-07 | 7.91e-06 | Acetone |

**(b) scaling to creatinine**

| **Spec. pos. [ppm]** | $\log_2$ **FC** | ***t*-value** | **raw *p*-value** | **B/H adj. *p*-value** | **Metabolite** |
|---|---|---|---|---|---|
| 1.395 | 0.90 | 6.71 | 9.28e-10 | 5.19e-07 | Tranexamic acid |
| 1.375 | 1.13 | 6.57 | 1.80e-09 | 5.19e-07 | Tranexamic acid |
| 1.045 | 1.24 | 6.52 | 2.23e-09 | 5.19e-07 | Tranexamic acid |
| 1.825 | 0.98 | 6.18 | 1.16e-08 | 1.98e-06 | Tranexamic acid |
| 1.025 | 1.06 | 6.13 | 1.42e-08 | 1.98e-06 | Tranexamic acid |
| 1.845 | 0.98 | 6.06 | 1.96e-08 | 2.29e-06 | Tranexamic acid |
| 1.065 | 1.03 | 5.92 | 3.77e-08 | 3.77e-06 | Tranexamic acid |
| 1.355 | 0.95 | 5.87 | 4.72e-08 | 4.13e-06 | Tranexamic acid/2-Hydroxyisobutyric acid |
| 1.055 | 0.99 | 5.82 | 6.10e-08 | 4.22e-06 | Tranexamic acid |
| 1.385 | 1.01 | 5.81 | 6.40e-08 | 4.22e-06 | Tranexamic acid |

**(c) PQN**

| **Spec. pos. [ppm]** | $\log_2$ **FC** | ***t*-value** | **raw *p*-value** | **B/H adj. *p*-value** | **Metabolite** |
|---|---|---|---|---|---|
| 2.475 | -0.52 | -6.47 | 2.92e-09 | 1.89e-06 | Carnitine/Glutamine |
| 2.465 | -0.56 | -6.34 | 5.39e-09 | 1.89e-06 | Carnitine/2-Oxoglutaric acid/Glutamine |
| 2.485 | -0.54 | -5.97 | 3.13e-08 | 7.31e-06 | Carnitine/Glutamine/Acetyl-L-carnitine |
| 1.395 | 0.52 | 5.77 | 7.84e-08 | 1.37e-05 | Tranexamic acid |
| 2.605 | -0.39 | -5.36 | 4.76e-07 | 6.67e-05 | Unknown |
| 2.615 | -0.40 | -5.16 | 1.12e-06 | 1.13e-04 | Unknown |
| 1.025 | 0.67 | 5.16 | 1.13e-06 | 1.13e-04 | Tranexamic acid |
| 1.375 | 0.74 | 5.12 | 1.37e-06 | 1.17e-04 | Tranexamic acid |
| 1.045 | 0.85 | 5.09 | 1.50e-06 | 1.17e-04 | Tranexamic acid |
| 2.495 | -0.53 | -5.05 | 1.84e-06 | 1.29e-04 | Acetyl-L-carnitine/Glutamine/Unknown |

Table 2: Spectral positions and $p$-values of the ten most significant NMR buckets for the plasma AKI data set after (a) scaling to total spectral area, (b) Probabilistic Quotient Normalization (PQN), and (c) scaling to TSP. The FDR was adjusted according to the method of Benjamini and Hochberg (B/H). In case more than one compound contributed to one significant bin, all possibly corresponding molecules are annotated.

**(a) scaling to total spectral area**

| Spec. pos. [ppm] | $\log_2$ FC | $t$-value | raw $p$-value | B/H adj. $p$-value | Metabolite |
|---|---|---|---|---|---|
| 7.285 | 1.37 | 7.71 | 2.10e-11 | 1.47e-08 | Propofol-glucuronide/Tryptophan |
| 4.305 | 1.24 | 7.57 | 3.98e-11 | 1.47e-08 | Multiple compounds |
| 3.625 | -0.44 | -7.28 | 1.49e-10 | 3.68e-08 | Free EDTA |
| 7.275 | 0.90 | 6.94 | 7.23e-10 | 1.34e-07 | Tryptophan/Propofol-glucuronide |
| 1.165 | 1.04 | 6.83 | 1.18e-09 | 1.75e-07 | 4-Hydroxy-propofol-1-OH-D-glucuronide/ Propofol-glucuronide/Isopropanol |
| 4.315 | 1.28 | 6.66 | 2.56e-09 | 3.15e-07 | Multiple compounds |
| 4.295 | 0.66 | 6.48 | 5.57e-09 | 5.89e-07 | Multiple compounds |
| 1.385 | 0.91 | 6.35 | 1.01e-08 | 9.38e-07 | Tranexamic acid |
| 4.015 | 0.58 | 6.17 | 2.16e-08 | 1.78e-06 | Isopropanol/Unknown |
| 3.285 | 0.47 | 6.03 | 4.07e-08 | 3.01e-06 | Myo-inositol/D-glucuronic acid (?)/ Phenylalanine/ 4-Hydroxy-propofol-4-OH-D-glucuronide |

**(b) PQN**

| Spec. pos. [ppm] | $\log_2$ FC | $t$-value | raw $p$-value | B/H adj. $p$-value | Metabolite |
|---|---|---|---|---|---|
| 3.625 | -0.57 | -8.48 | 5.88e-13 | 4.35e-10 | Free EDTA |
| 7.285 | 1.24 | 7.42 | 7.91e-11 | 2.93e-08 | Propofol-glucuronide/Tryptophan |
| 4.305 | 1.11 | 7.12 | 3.14e-10 | 7.75e-08 | Multiple compounds |
| 7.275 | 0.77 | 6.59 | 3.48e-09 | 6.44e-07 | Tryptophan/Propofol-glucuronide |
| 1.165 | 0.92 | 6.52 | 4.72e-09 | 6.99e-07 | 4-Hydroxy-propofol-1-OH-D-glucuronide/ Propofol-glucuronide/Isopropanol |
| 3.105 | -0.23 | -6.36 | 9.40e-09 | 1.16e-06 | $CaEDTA^{2-}$ |
| 4.315 | 1.15 | 6.23 | 1.68e-08 | 1.77e-06 | Multiple compounds |
| 3.335 | -0.18 | -6.05 | 3.69e-08 | 3.41e-06 | Unknown/Proline (?)/Tryptophan |
| 3.165 | -0.22 | -5.97 | 5.25e-08 | 4.32e-06 | $CaEDTA^{2-}$ |
| 1.385 | 0.79 | 5.92 | 6.61e-08 | 4.89e-06 | Tranexamic acid |

**(c) scaling to TSP**

| Spec. pos. [ppm] | $\log_2$ FC | $t$-value | raw $p$-value | B/H adj. $p$-value | Metabolite |
|---|---|---|---|---|---|
| 7.285 | 1.45 | 7.80 | 1.40e-11 | 1.04e-08 | Propofol-glucuronide/Tryptophan |
| 4.305 | 1.32 | 7.35 | 1.09e-10 | 4.05e-08 | Multiple compounds |
| 7.275 | 0.98 | 6.97 | 6.15e-10 | 1.49e-07 | Tryptophan/Propofol-glucuronide |
| 1.165 | 1.12 | 6.91 | 8.05e-10 | 1.49e-07 | 4-Hydroxy-propofol-1-OH-D-glucuronide/ Propofol-glucuronide/Isopropanol |
| 4.315 | 1.36 | 6.61 | 3.19e-09 | 4.72e-07 | Multiple compounds |
| 2.815 | 0.38 | 6.44 | 6.83e-09 | 8.43e-07 | Unknown |
| 3.285 | 0.55 | 6.39 | 8.35e-09 | 8.83e-07 | Myo-inositol/D-glucuronic acid (?)/ Phenylalanine/ 4-Hydroxy-propofol-4-OH-D-glucuronide |
| 3.625 | -0.36 | -6.32 | 1.13e-08 | 1.05e-06 | Free EDTA |
| 2.765 | 0.28 | 6.29 | 1.29e-08 | 1.06e-06 | Unknown |
| 1.385 | 0.99 | 6.23 | 1.71e-08 | 1.26e-06 | Tranexamic acid |

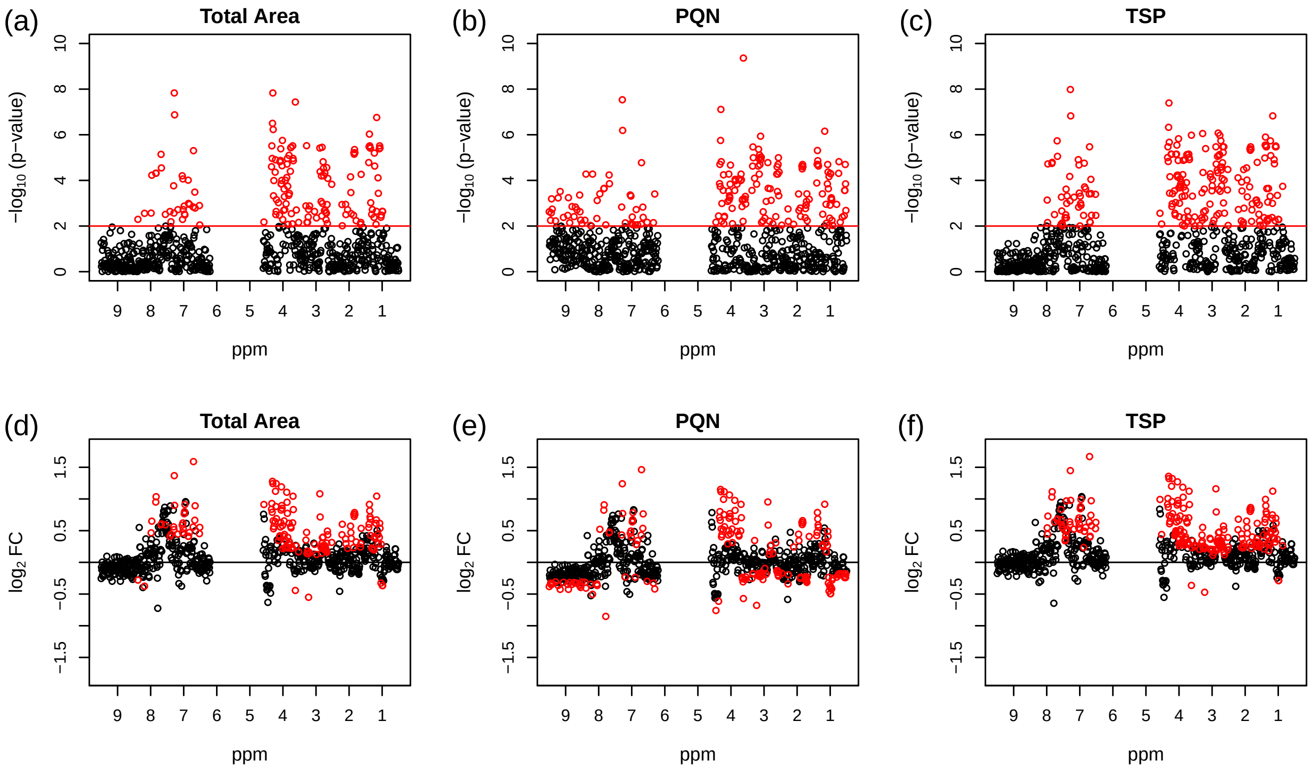


Figure 1: $-\log_{10}(p\text{-values})$ of moderated $t$-test analysis comparing healthy versus diseased patients for the plasma AKI data set after preprocessing with three different normalization methods, i.e., (a) scaling to equal total spectral area, (b) PQN, or (c) scaling to TSP, respectively, plotted versus the ppm regions of the corresponding NMR features (upper figure). A red line marks the significance level for Benjamini-Hochberg (B/H) adjusted $p$-values below 0.01, corresponding to a false discovery rate (FDR) below 1%. All NMR features with a B/H-adjusted $p$-value below 0.01 are represented as red dots. The lower figures, (e - h), show the corresponding $\log_2$(fold-changes) ($\log_2$ FC) versus the ppm regions of the corresponding NMR features. $\log_2$ FCs were calculated as AKI minus non-AKI, thus positive $\log_2$ FCs correspond to higher values in AKI than in non-AKI.

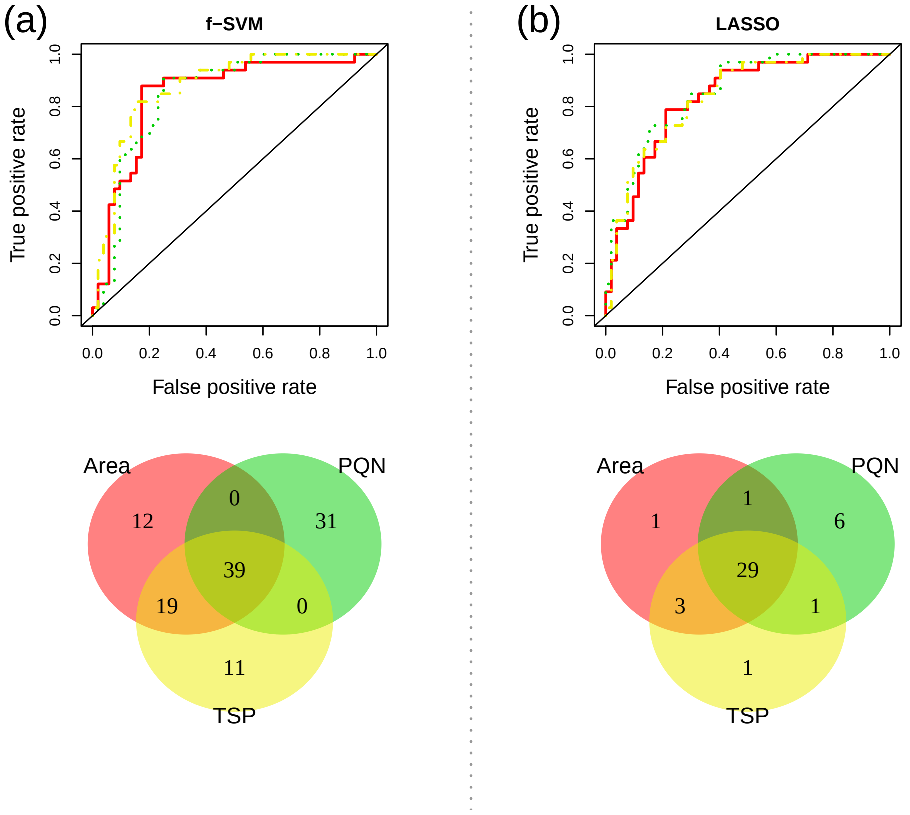


Figure 2: The plasma AKI data set: Receiver operating characteristic (ROC) curves for two classification approaches, (a) SVM in combination with $t$-test based feature filtering, and (b) LASSO, after application of three different normalization strategies: scaling to total spectral area (red solid line), Probabilistic Quotient Normalization (PQN) (green dotted line), and scaling to TSP (yellow dashed-dotted line). The bottom row shows the number of features included in the respective classification models in Venn diagrams. The corresponding models were built by averaging over all models of the outer CV loop.

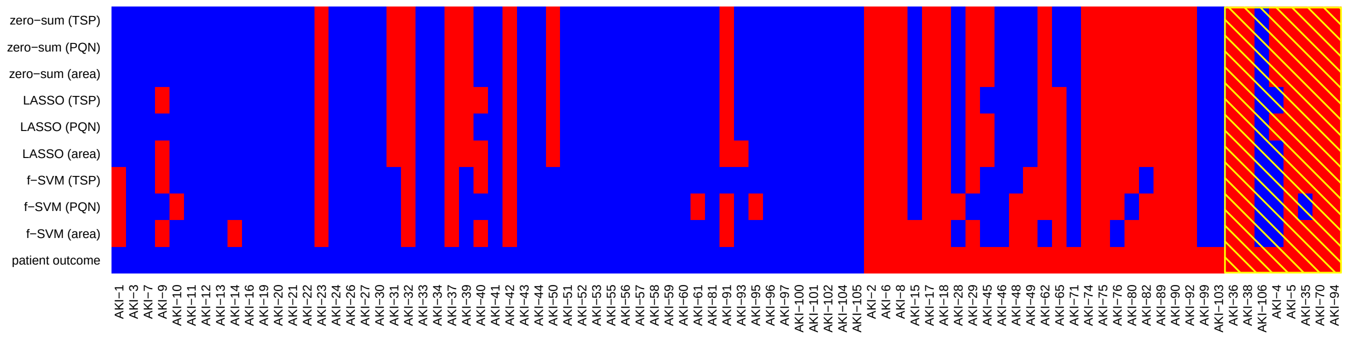


Figure 3: Classification results patient by patient for the plasma AKI data set: The row “patient outcome” shows patients that did not develop AKI in blue, patients that developed AKI in red, while patients that developed severe AKI (AKIN stage 2 and 3) are further highlighted by the yellow dashed region. Above we give predictions for the onset of AKI for f-SVM, LASSO, and zero-sum, using normalization strategies as indicated in brackets. AKI predictions are shown in red (AKIN stages 1 to 3), while patients predicted as non-AKI are shown in blue.
